# Supplementary material for: Evaluation of RAG Metrics for Question Answering in the Telecom Domain
Source: arXiv:2407.12873 source file (2024-07-15)
Supplement: Supplementary file 1 [file ques_table_appendix.tex]

\begin{table}[H]
\centering
\scalebox{0.98}{
\begin{tabular}{|p{0.2\linewidth}|p{0.35\linewidth}p{0.35\linewidth}|}
\hline
\multicolumn{1}{|c|}{\textbf{RAG Response/Metrics}} & \multicolumn{2}{c|}{\textbf{Question/Answer and Supporting Statements for RAGAS Metrics}}                                                                                                                                                                                                                                                                                                                                                                                                                                                                                                                                                                                                                                                                                                                                                                                                                                                                                                                                                                                                                       \\ \hline
\rowcolor[HTML]{d9d7d4}
Question \& Ground Truth                   & \multicolumn{1}{C{0.4\linewidth}|}{Question: What is the optional output for Ngmlc\_Location\_LocationUpdate?}                                                                                                                                                                                                                                                                                                                                                                                                                                                                 & Answer: "Failure Cause (in the case of failure indication provided)",                                                                                                                                                                                                                                                                                                                                                                                                                                                                \\ \hline
RAG Response                               & \multicolumn{2}{C{0.75\linewidth}|}{"NO ANSWER FOUND. The given context only mentions the required and optional inputs for the Ngmlc\_Location\_LocationUpdate service operation, but it does not provide information about the optional output."}                                                                                                                                                                                                                                                                                                                                                                                                                                                                                                                                                                                                                                                                                                                                                                                                                                                                     \\ \hline
\multirow{3}{*}{Faithfulness: 0}    & \multicolumn{2}{C{0.75\linewidth}|}{Statements: "NO ANSWER FOUND. The given context only mentions the required and optional inputs for the Ngmlc\_Location\_LocationUpdate service operation, but it does not provide information about the optional output."}                                                                                                                                                                                                                                                                                                                                                                                                                                                                                                                                                                                                                                                                                                                                                                                                                                                         \\ \cline{2-3} 
                                           & \multicolumn{2}{C{0.75\linewidth}|}{Explanation: The given context specifies the required inputs and optional outputs for the Ngmlc\_Location\_LocationUpdate service operation. The required inputs are UE identifier (GPSI or SUPI), identity of the AF, event causing the location estimate (5GC-MO-LR), location estimate, age of location estimate, and accuracy indication. The optional outputs are Success/Failure indication and Failure Cause.\textbackslash{}n\textbackslash{}nVerdict: False. The context does mention optional outputs for the Ngmlc\_Location\_LocationUpdate service operation., "Explanation: The context description mentions that the optional output for Ngmlc\_Location\_LocationUpdate includes a \textbackslash{}"Failure Cause (in the case of failure indication provided)\textbackslash{}". However, it does not provide any specific information about other potential optional outputs.\textbackslash{}n\textbackslash{}nVerdict: Partially false. The context does mention one optional output, but it does not provide information about all possible optional outputs."} \\ \cline{2-3} 
                                           & \multicolumn{2}{l|}{Verdicts: false, false}                                                                                                                                                                                                                                                                                                                                                                                                                                                                                                                                                                                                                                                                                                                                                                                                                                                                                                                                                                                                                                                            \\ \hline
Ans Correctness: 0               & \multicolumn{2}{C{0.75\linewidth}|}{Output: \{\textbackslash{}FP\textbackslash{}": {[}{]}, \textbackslash{}"TP\textbackslash{}": {[}{]}, \textbackslash{}"FN\textbackslash{}": {[}\textbackslash{}"Failure Cause (in the case of failure indication provided)\textbackslash{}"{]}\}", "num\_tp": 0, "num\_fp": 0, "num\_fn": 1}                                                                                                                                                                                                                                                                                                                                                                                                                                                                                                                                                                                                                                                                                                                                                                                        \\ \hline
Context Relevance: 0.16        & \multicolumn{2}{C{0.75\linewidth}|}{Statements:         "Output, Optional: Failure Cause (in the case of failure indication provided)."}                                                                                                                                                                                                                                                                                                                                                                                                                                                                                                                                                                                                                                                                                                                                                                                                                                                                                                                                                                               \\ \hline \hline
\rowcolor[HTML]{d9d7d4} 
Question \& Ground Truth                   & \multicolumn{1}{C{0.4\linewidth}|}{Question: "What bandwidth is suitable to 6 paths in SCSM model?"}                                                                                                                                                                                                                                                                                                                                                                                                                                                                  & Answer: "5MHz"                                                                                                                                                                                                                                                                                                                                                                                                                                                                                                        \\ \hline
RAG Response                               & \multicolumn{2}{C{0.75\linewidth}|}{"NO ANSWER FOUND. The provided text does not mention the bandwidth suitable for 6 paths in the SCSM (Stochastic Channel Model) model. The text only mentions that the SCM model described with N = 6 paths may not be suitable for systems with bandwidth higher than 5MHz."}                                                                                                                                                                                                                                                                                                                                                                                                                                                                                                                                                                                                                                                                                                                                                                                                      \\ \hline
                                           & \multicolumn{2}{C{0.75\linewidth}|}{Statements: No answer was found in the text regarding the bandwidth suitable for 6 paths in the SCSM model., "The text mentions that an SCM model with N = 6 paths may not be suitable for systems with bandwidth higher than 5MHz."}                                                                                                                                                                                                                                                                                                                                                                                                                                                                                                                                                                                                                                                                                                                                                                                                                                              \\ \cline{2-3} 
                                           & \multicolumn{2}{C{0.75\linewidth}|}{Explanation: Yes, the text does not provide information on the suitable bandwidth for 6 paths in the SCSM model. The text only mentions that the SCM model described with N = 6 paths may not be suitable for systems with bandwidth higher than 5MHz, but it does not specify the exact bandwidth for which the given pathloss equations are valid., "Yes, the context mentions that the SCM model with N = 6 paths may not be suitable for systems with bandwidth higher than 5MHz (Clause 5.6.2). The context explains that this model may not be accurate for wider bandwidths and suggests using other models for such cases."}                                                                                                                                                                                                                                                                                                                                                                                                                                               \\ \cline{2-3} 
\multirow{-3}{*}{Faithfulness: 1}          & \multicolumn{2}{C{0.75\linewidth}|}{Verdicts: true, true}                                                                                                                                                                                                                                                                                                                                                                                                                                                                                                                                                                                                                                                                                                                                                                                                                                                                                                                                                                                                                                                              \\ \hline
Ans Correctness: 0.66                      & \multicolumn{2}{C{0.75\linewidth}|}{\{\textbackslash{}FP\textbackslash{}": {[}{]}, \textbackslash{}"TP\textbackslash{}": {[}\textbackslash{}"The SCM model with N = 6 paths may not be suitable for systems with bandwidth higher than 5MHz\textbackslash{}"{]}, \textbackslash{}"FN\textbackslash{}": {[}\textbackslash{}"5MHz is the bandwidth suitable for 6 paths in SCSM model\textbackslash{}"{]}\}", "num\_tp": 1, "num\_fp": 0, "num\_fn": 1}                                                                                                                                                                                                                                                                                                                                                                                                                                                                                                                                                                                                                                                                  \\ \hline
Context Relevance: 0.0                     & \multicolumn{2}{C{0.75\linewidth}|}{None}                                                                                                                                                                                                                                                                                                                                                                                                                                                                                                                                                                                                                                                                                                                                                                                                                                                                                                                                                                                                                                                                              \\ \hline \hline

\end{tabular}
}
\end{table}
